# Supplementary material for: Historia: Refuting Callback Reachability with Message-History Logics (Extended Version)
Source: arXiv:2309.04464 source file (2023-09-11)
Supplement: Supplementary file 2 [file appendix_appendix.tex]

%\section{Code listings for simplified examples}
%\label{sec:codelist}
%\paragraph{Antennapod 2856}
%\begin{lstlisting}[language=Java,alsolanguage=exthighlighting,style=number]
%public class PlayerFragment 
%    extends Fragment implements Action1<Object>{
%  Subscription sub;
%  @Override
%  public void onCreate(Bundle s){
%    sub = Single.create(subscriber -> {
%      subscriber.onSuccess(3);
%    }).subscribe(this);
%  }
%
%  @Override
%  public void call(Object o){
%     Activity act = getActivity(); 
%     assert(act != null);
%     act.toString();
%  }
%
%  @Override
%  public void onDestroy(){
%    sub.unsubscribe();
%  }
%}
%\end{lstlisting}
%
%\paragraph{Antennapod 1306}
%\begin{lstlisting}[language=Java,alsolanguage=exthighlighting,style=number]
%public class RemoverActivity 
%		extends Activity 
%		implements OnClickListener{
%    FeedRemover remover = null;
%    View button = null;
%    @Override
%    public void onCreate(Bundle b){
%        remover = new FeedRemover();
%        button = findViewById(3);
%        button.setOnClickListener(this);
%    }
%    @Override
%    public void onClick(View v){
%        remover.execute();
%        button.setEnabled(false);
%    }
%
%
%    class FeedRemover 
%      extends AsyncTask<String, Void, String> {
%	  @Override
%	  protected void onPreExecute() {}
%	  @Override
%	  protected String doInBackground(String... p) {
%		  return "";
%	  }
%	  @Override
%	  protected void onPostExecute(String r) {
%        RemoverActivity.this.finish();
%	  }
%  }
%}
%\end{lstlisting}
\iffalse
\section{Well Formed Constraints for \newls}
\begin{mathpar}
\fbox{
      \wellformed{\directive}
      \\
      \wellformedU{\directive}
    }

    \infer[]{ }{\wellformed{\iDir{\ltmsg}}}

    \infer[]{ }{\wellformed{\niDir{\ltmsg_1}{\ltmsg_2}}}
  
    \infer[]{ \wellformed{\directive}}{
      \wellformed{\exists \symval.~\directive}
    }

    \infer[]{\wellformed{\directive}\wedge\wellformed{\directive'}}{
      \wellformed{\directive \wedge \directive'}
    }

    \infer[]{\wellformed{\directive}\vee\wellformed{\directive'}}{
      \wellformed{\directive \vee \directive'}
    }

    \infer[]{ \wellformedU{\directive}}{
      \wellformed{\forall \symval.~\directive}
    }

    \infer[]{ \wellformedU{\directive}}{
      \wellformed{\directive}
    }

    \infer[]{ }{\wellformedU{\notiDir{\ltmsg}}}

    \infer[]{\wellformedU{\directive}\wedge\wellformedU{\directive'}}{
      \wellformedU{\directive \wedge \directive'}
    }

    \infer[]{\wellformedU{\directive}\vee\wellformedU{\directive'}}{
      \wellformedU{\directive \vee \directive'}
    }

    \infer[]{ }{
      \wellformedU{\absof{x} = \absof{y}}
    }

    \infer[]{ }{
      \wellformedU{\absof{x} \neq \absof{y}}
    }

    \infer[]{ }{
      \wellformedU{\text{true}}
    }

    \infer[]{ }{
      \wellformedU{\text{false}}
    }
\end{mathpar}
\fi
\section{What do we express with \newls?}
\label{sec:newlsdesign}
\TODO{This was a subsection of \newls, some of the content should be merged back into that section, but the specs should probably remain in the appendix}

A \newls formula $\SpecSet$ expresses a set of message histories. However, $\SpecSet$ does not need to express the complete framework model but only ``what is sufficient'' to refute a goal query.
As we described in~\secref{overview}, a developer starts the specification loop with the most permissive set of message histories (i.e., the ``top model'' $\SpecSet = \text{true}$), and then refine such formula iteratively.
Here, we explain how such use case motivates the \newls's design.

\paragraph{Targeted specification of message history}\TODO{targeted still applies here}
The program analysis provides a sequence of callbacks that may reach a goal query and the developer uses such counter example to refine the \newls formula $\SpecSet$.
The temporal operators of \newls allows a developer to express a restriction on the message history every time a specific message from the counter example happens.
Consider again specification~\ref{spec:callsubonly}\TODO{removed, update this}:
\[
   \speccb{\codej{l}}{call}{} \boxright \iDir{\specci{\codej{_}}{subscribe}{\codej{l}}}.
\]

stating that "every time a listener object \codej{l} invokes \codej{call}, there is an object \codej{k} that subscribed \codej{l} in the past".
The top-level temporal operator in the logic, history implication ($\boxright$), expresses that the formula $\iDir{\enkwCi~(\exists\ \codej{k}.\ \codej{k.subscribe(l)})}$ holds in the message history \emph{before} \codej{call} (underscore is syntactic sugar for a variable not captured by the specification and expands to introduce a unique existential variable, $k$).
The past temporal operator $\iDir{\enkwCi~(\exists\ \codej{k}.\ \codej{k.subscribe(l)})}$ then restricts the message history.
That's it, each specification, \ltrule, is goal-directed and expresses the effect a single message has on the message history.
%
% [Sergio] Not explained: why a single message and not more?
%

The combination of the history implication and the past temporal operators ($\iDir{}$ - \emph{Once}, $\notiDir{}$ - \emph{Historically Not}, and $\niDir{}{}$ - \emph{Not Since}) expresses common usage patterns of callbacks and callins.
The rule $\specOnly{\absmsg}{\iDir{\ltmsg}}$ expresses that an invocation of $\absmsg$ is always preceded by the invocation of $\ltmsg$, as in the case of the callback \codej{call} and the registration of the listener object \codej{subscribe}.
Similarly, $\specOnly{\absmsg}{\notiDir{\ltmsg}}$ states that $\absmsg$ is never preceded by $\ltmsg$. An instance of such pattern is specification \ref{spec:createOnce}: every invocation of the \codej{onCreate} method must not be preceded by the same invocation (i.e., with the same receiver object) of \codej{onCreate}.
The specification $\specOnly{\absmsg}{\niDir{\ltmsg_1}{\ltmsg_2}}$ states that $\absmsg$ is always preceded by $\ltmsg_2$, with no invocations of $\ltmsg_1$ in between. Such pattern captures that an invocation of $\ltmsg_1$ would prevent the invocation of $\absmsg$. For example, specification~\ref{spec:call} expresses that the message \codej{subscribe} has been invoked more recently than the \codej{unsubscribe} callin.

\paragraph{Refining the message history compositionally}
Developers refine the formula $\SpecSet$ iteratively. Consider Specification \ref{spec:clickFinish}.
A separate behavior of the \codej{onClick} callback is that if the associated button is disabled via \codej{setEnabled(false)}, then the \codej{onClick} callback cannot occur (Specification \ref{spec:clickDisable}).

The developer can conjunct the specification \ref{spec:clickDisable} with the specification \ref{spec:clickFinish}, refining the set of message histories when the \codej{onClick} callback occurs.
The syntax of \newls where a formula $\SpecSet$ is a conjunction of specifications only allows the developer to refine an existing specification (or, in logical terms, strengthen a formula $\SpecSet$).
This way, the developer would start from the ``most permissive'' and sound specification $\SpecSet = \text{true}$, and \emph{compositionally} refine $\SpecSet$ as needed for the messages appearing in a counter example.

\paragraph{Expressing parameter binding across messages}
As we have seen in the previous specifications, \newls can express the binding of parameters across messages using universal and existential quantifiers.
A significant example of parameter bindings across different messages is specification \ref{spec:clickFinish}, which captures the behavior of the \codej{onClick} callback.
Such specification captures the interaction of multiple objects. For \codej{onClick} to occur on a listener object \codej{l}, there must exist a \codej{Button} object \codej{v}, an \codej{Activity} object \codej{a}, and an integer \codej{m} such that:
\begin{inparaenum}
\item the listener \codej{l} has been registered to the button \codej{v} - observed with $\enkwCi~\codej{v.setOnClickList(l)}$; 
\item the button \codej{v} is attached to the Activity - observed by $\iDir{\enkwCi~\codej{v:=a.findViewById(m)}}$;
\item the Activity \codej{a} is neither paused nor has the application requested the activity finish; and
\item since the listener has been registered, \codej{setOnClickListener} has not been called with a null value.
\end{inparaenum}

Another example of the use of quantifiers is to express that the relationship between two objects is unique.  For example, the following specification relates a \codej{Button} and an \codej{Activity} object, expressing that the button can be attached to a single \codej{Activity} (Specification \ref{spec:findView}). 

\section{Empirical Evaluation - Additional Material}
\TODO{TO REVISE OR CUT!}

\subsection{Benchmark and Specification Description}
\label{sec:benchdescription}
\TODO{Still not revised - to evaluate if should be added as is or not in the appendix (this section has some specification linked from the main table)}

%To evaluate our technique, we select 4 crashes with stack traces in open source Android applications that cannot be handled by existing static analysis tools.  
%We then write a minimal set of specifications sufficient to prove the fixed version of the application.
Here, we describe how we chose these benchmarks, what the benchmarks are, and what specifications had to be written for them.
Each of these defects is witnessed by an unexpected ordering of callbacks associated with a mixture of background tasks, UI objects and lifecycle components.
Based on our survey of the literature, each of these components is deeply modeled by some tool.  However, to our knowledge, no other tool can reason precisely across these domains.
We show that relatively simple specifications may be used capturing some of the properties of each domain to prove the defect.

Background tasks are used to move long running tasks off the UI thread and maintain responsiveness of the UI.  For example, loading the media object in our motivating example.  In addition to \codej{Single}(\apGa) used in the introduction, we also have examples that use \codej{AsyncTask} (\ymDi, \apEx) and \codej{Handler}(\cbFi).  There are valid reasons, as a developer, to use one or another of these APIs.  For the purposes of proving safety, we care about the general pattern that they have a separate "long running" callback and upon completion, a callback to update the user interface.

Our benchmarks also include examples of apps that utilize UI objects. \codej{View} is a general class for multiple components including buttons (\apEx, \cbFi).  \codej{Dialog} is a popup window that appears over an app and may be used to indicate a running background task (\ymDi).  These share some general properties that they have callbacks indicating user behavior and often depend on the visibility state of the lifecycle object they are attached to.

Lifecycle components are a class of UI objects that respond to OS events such as creation, resuming, pausing, and destruction.  These include \codej{Fragment} and \codej{Activity}.  These objects have callbacks corresponding to state transitions and callins connecting them to UI objects.  All four of our examples use one of these two objects.

Several specifications used for these benchmarks have already been introduced by earlier sections (i.e. section \ref{sec:overview} introduces \ref{spec:call} and \ref{spec:createOnce} and section \ref{sec:newls} introduces \ref{spec:findView}, \ref{spec:clickDisable}, and \ref{spec:clickFinish}).  

\JEDI{Benchmark 1: motivating example}
The first benchmark, Antenna Pod pull request 2856 (\apGa), was simplified slightly for the introduction. 
The general idea of this benchmark is that the \codej{Fragment} object's lifecycle interacts with the background task, \codej{Single}.
In the intro, we elide a call to the \codej{getActivity} method and replaced it with a nullable field in the \codej{call} method.
Additionally, the callback \codej{onActivityCreated} is used instead of \codej{onCreate}.
\codej{getActivity} behaves similarly to the nullable \codej{act} field returning a null value before \codej{onActivityCreated} or after \codej{onDestroy}.
The fix is to use \codej{unsubscribe} when the \codej{Fragment} is going into the destroyed state.

We have already listed specification \ref{spec:call}.
In addition, we needed two more specifications, one for \codej{getActivity} and the second relates \codej{onActivityCreated} and \codej{onDestroy}.
The corresponding specification for non-null value version of \codej{getActivity} need not be written since a non-null value invalidates the premise of the implication and is trivially true (Specifications \ref{spec:getActivityNull} and \ref{spec:onActivityCreated}).

\JEDI{Benchmark 2: execute twice and button behavior}
The second benchmark, Antenna Pod pull request 1306 (\apEx), uses a background task \codej{AsyncTask} object which may only have \codej{execute} invoked once on any given instance.  
\codej{AsyncTask} is intended to be an object encapsulating a single, one time use task.  
The framework throws an exception because such a design may mean that the single use directive is violated \ref{spec:execute}.
The crash is a result of a \codej{onClick} callback that can be invoked twice if the user taps fast enough. 
This app was fixed by calling \codej{setEnabled(false)} on the button when clicked explained by \ref{spec:clickDisable}.
This benchmark also uses \ref{spec:createOnce}.

\JEDI{Benchmark 3: dismissing a dialog after a task completes}
The third benchmark, Yamba pull request 1 (\ymDi), uses a \codej{Dialog} object displayed when \codej{show} is invoked.
It is expected that the dialog is always attached to a lifecycle object, in this case \codej{Activity}, this association is set as a parameter of the \codej{show} method.
An \codej{AsyncTask} invokes a callback upon completion invoking \codej{dismiss} on the dialog.  
If the associated \codej{Activity} is in the paused state, an exception occurs. 
The fix was to create a boolean field to track the resumed state of the \codej{Activity} and check before invoking \codej{dismiss}.
Since such a check does not rely on the state of the \codej{AsyncTask}, no specifications on \codej{AsyncTask} were necessary.
%The two specs required were \ref{spec:show} and \ref{spec:dismiss}.  
This crash was from the running example of a textbook on programming Android apps motivating how hard such reasoning can be~\cite{Gargenta:2014aa}.

\JEDI{Benchmark 4: the finish method and violation of the onClick while active assumption}

The fourth benchmark, Connect Bot pull request 1015 (\cbFi), crashes because a \codej{onClick} callback may occur after the \codej{Activity} has been paused invoking \codej{onPause}.  This click is possible because the Activity is put into the finishing state because the app invoked \codej{finish}.  
This strange behavior between \codej{Activity}, \codej{onClick}, and \codej{finish} is described by \citet{DBLP:conf/ecoop/MeierMC19} and captured by the specification \ref{spec:clickFinish}.
However, app developers and program analysts must work with the framework they are given.

The 4th application, Connect Bot, did not have a fix. 
We iterated specifications on the buggy version of Connect Bot until we had an alarm and witness that explained the crash and subsequently issued a pull request to fix the defect.
In order to avoid an alarm on the fixed version, we invoked \codej{v.setOnClickListener(null)} when finishing to prevent a future click.
Our fix was accepted by the maintainers of the Connectbot project adding confidence that this is the correct fix.

In order to write a specification for our fix, we needed three specifications:
\begin{inparaenum}
\item A strengthened specification \ref{spec:clickFinish} capturing the \codej{v.setOnClickListener(null)} behavior.
\item specification \ref{spec:findView} to state that the button retrieved from this \codej{Activity} may not be retrieved by a different activity, and
\item specification \ref{spec:createOnce} from the first benchmark.
\end{inparaenum}
These were sufficient to prove the fix safe to a depth of 5 callbacks.  However, the added complexity prevented our algorithm proving safety for an arbitrary number of callbacks.

\subsection{Additional Implementation Details}
Our implementation is built on the Soot analysis framework \cite{vall99soot} to load an APK, instrument the framework, and generate an initial points-to analysis.  
Our application memory abstraction is based on separation logic where abstract values are constrained by allocation sites, this technique closely mirrors the techniques of \citet{DBLP:conf/pldi/BlackshearCS13}. 

We generate a points to analysis using Spark from the Soot analysis framework. An artificial main method is generated and instrumented such that it may
\begin{inparaenum}
\item allocate any framework object and add them to the framework store,
\item allocate entry point objects in the application (these are typically declared in xml configuration files and reflectively instantiated in the actual framework) and add them to the framework store,
\item call any callback with a value from the framework store
\end{inparaenum}.
Additionally, we instrument all callins such that the arguments are written to the framework store and return values are chosen from the framework store.
This gives us an initial points-to analysis based on similar principles to the call graph described by \cite{DBLP:conf/ecoop/AliL12}.

\subsection{Scalability of the Entailment Judgment}
Entailment checking is much slower than other operations dispatched to the SMT solver, this likely corresponds to not being in the decidable fragment of logic discussed earlier.

Figure \ref{fig:hist} plots a histogram for both feasibility and entailment checks that are dispatched to the SMT solver.  
All feasibility checks finish in under 2 seconds and the vast majority finish in under a quarter of a second.  

For entailment, the vast majority of calls to the SMT solver finish in under 2 minutes.  However, when the subsumption check cannot finish in a reasonable amount of time, we must assume that the state cannot be subsumed to be sound.  Therefore, a small number of timeouts during subsumption checking can dramatically increase the number of explored states.  We suspect that a combination of the time spent checking entailment and the extra states inmtroduced by lack of subsumption is preventing us from proving the Connectbot benchmark to an arbitrary depth.

\begin{figure}[H]
\includegraphics[scale=0.30]{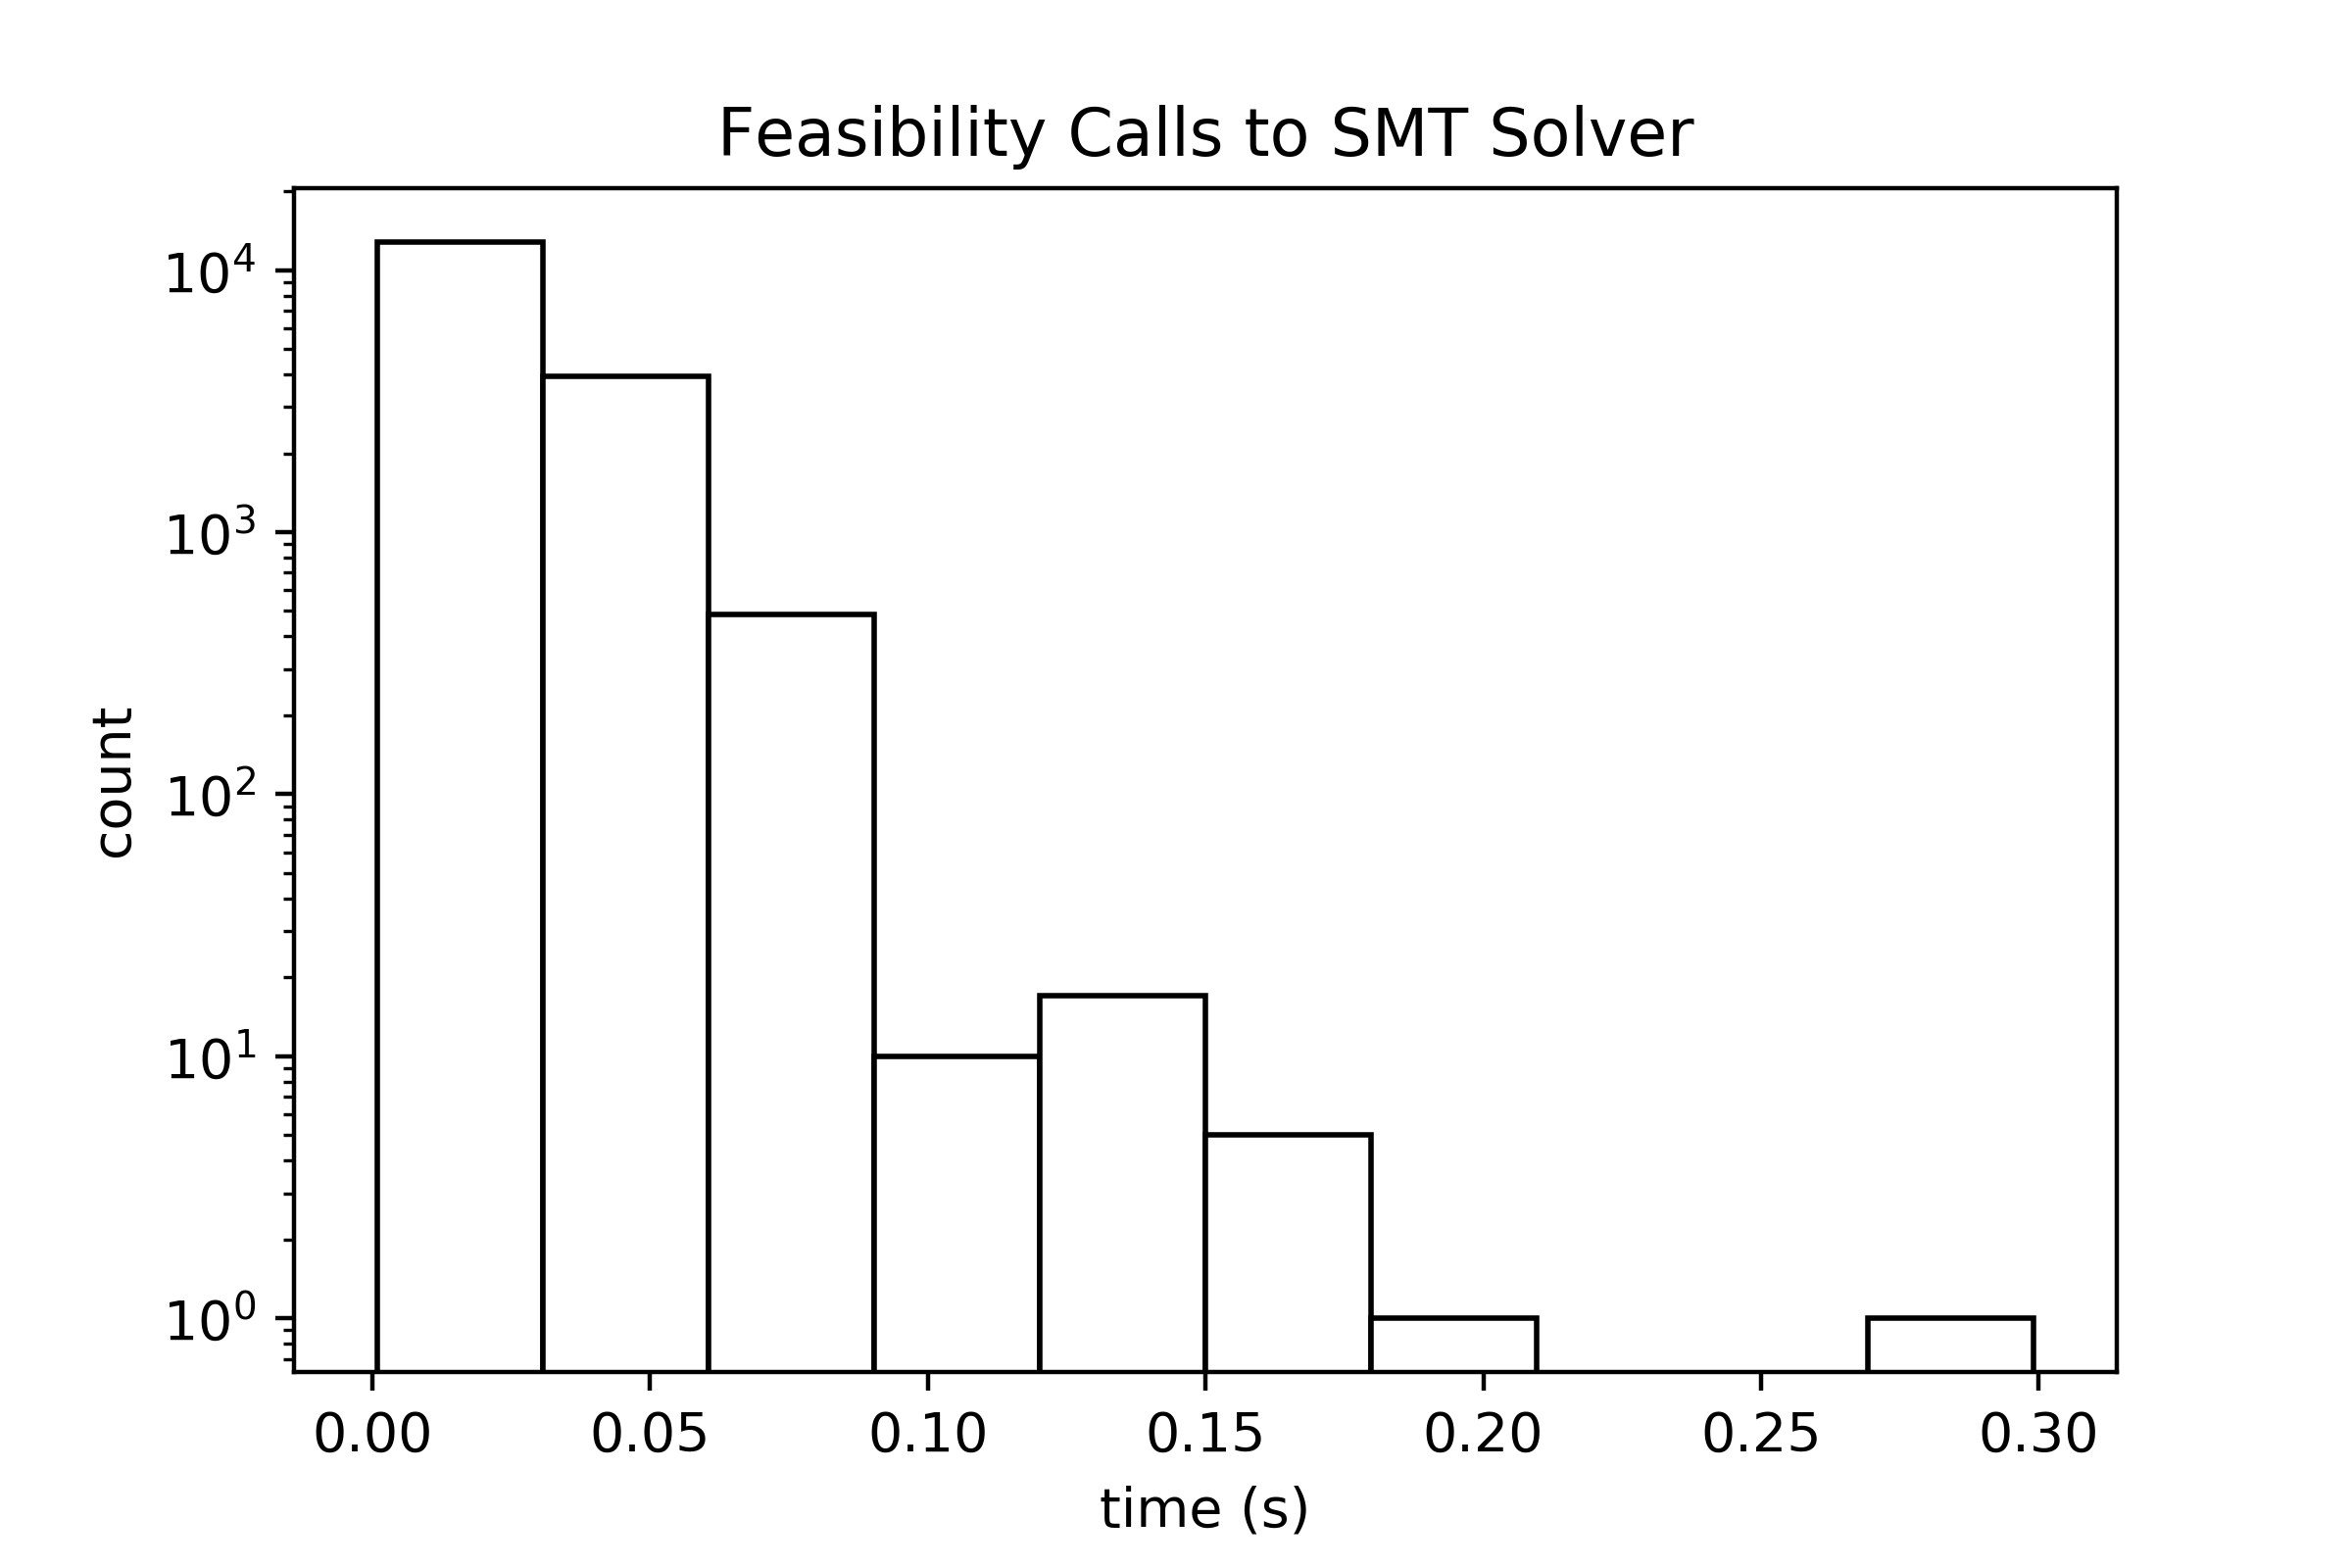}%
\includegraphics[scale=0.30]{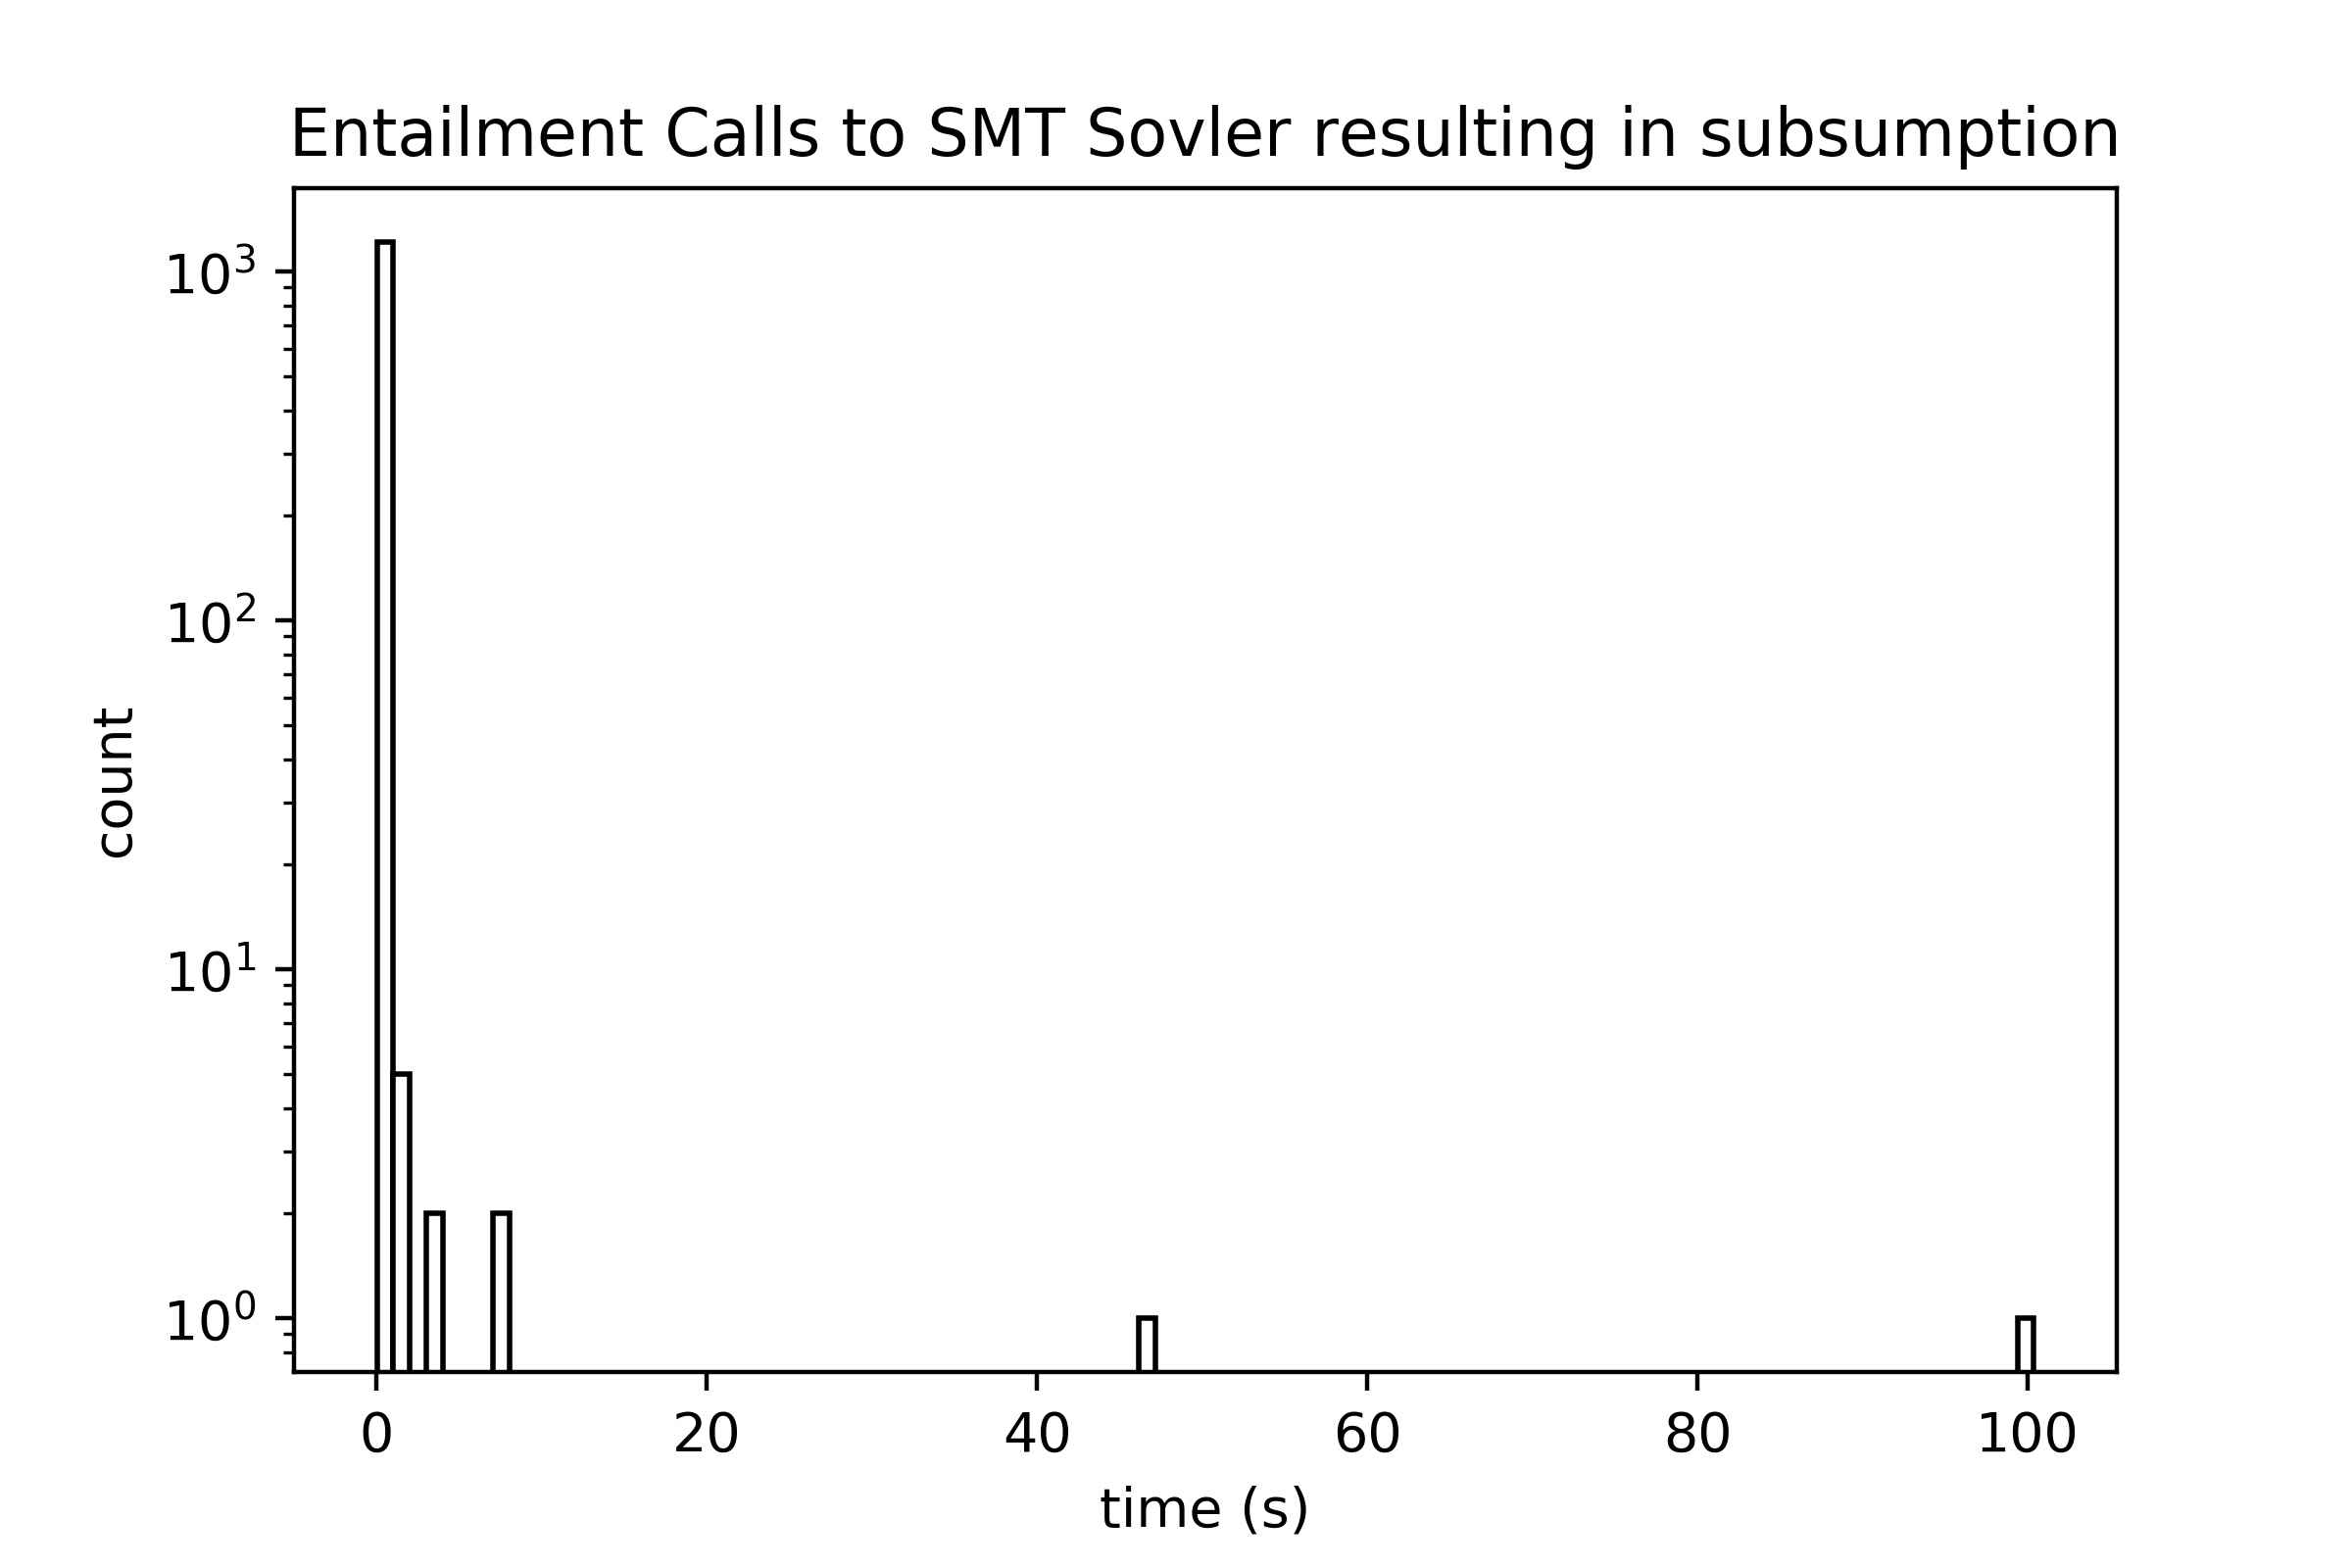}
\includegraphics[scale=0.30]{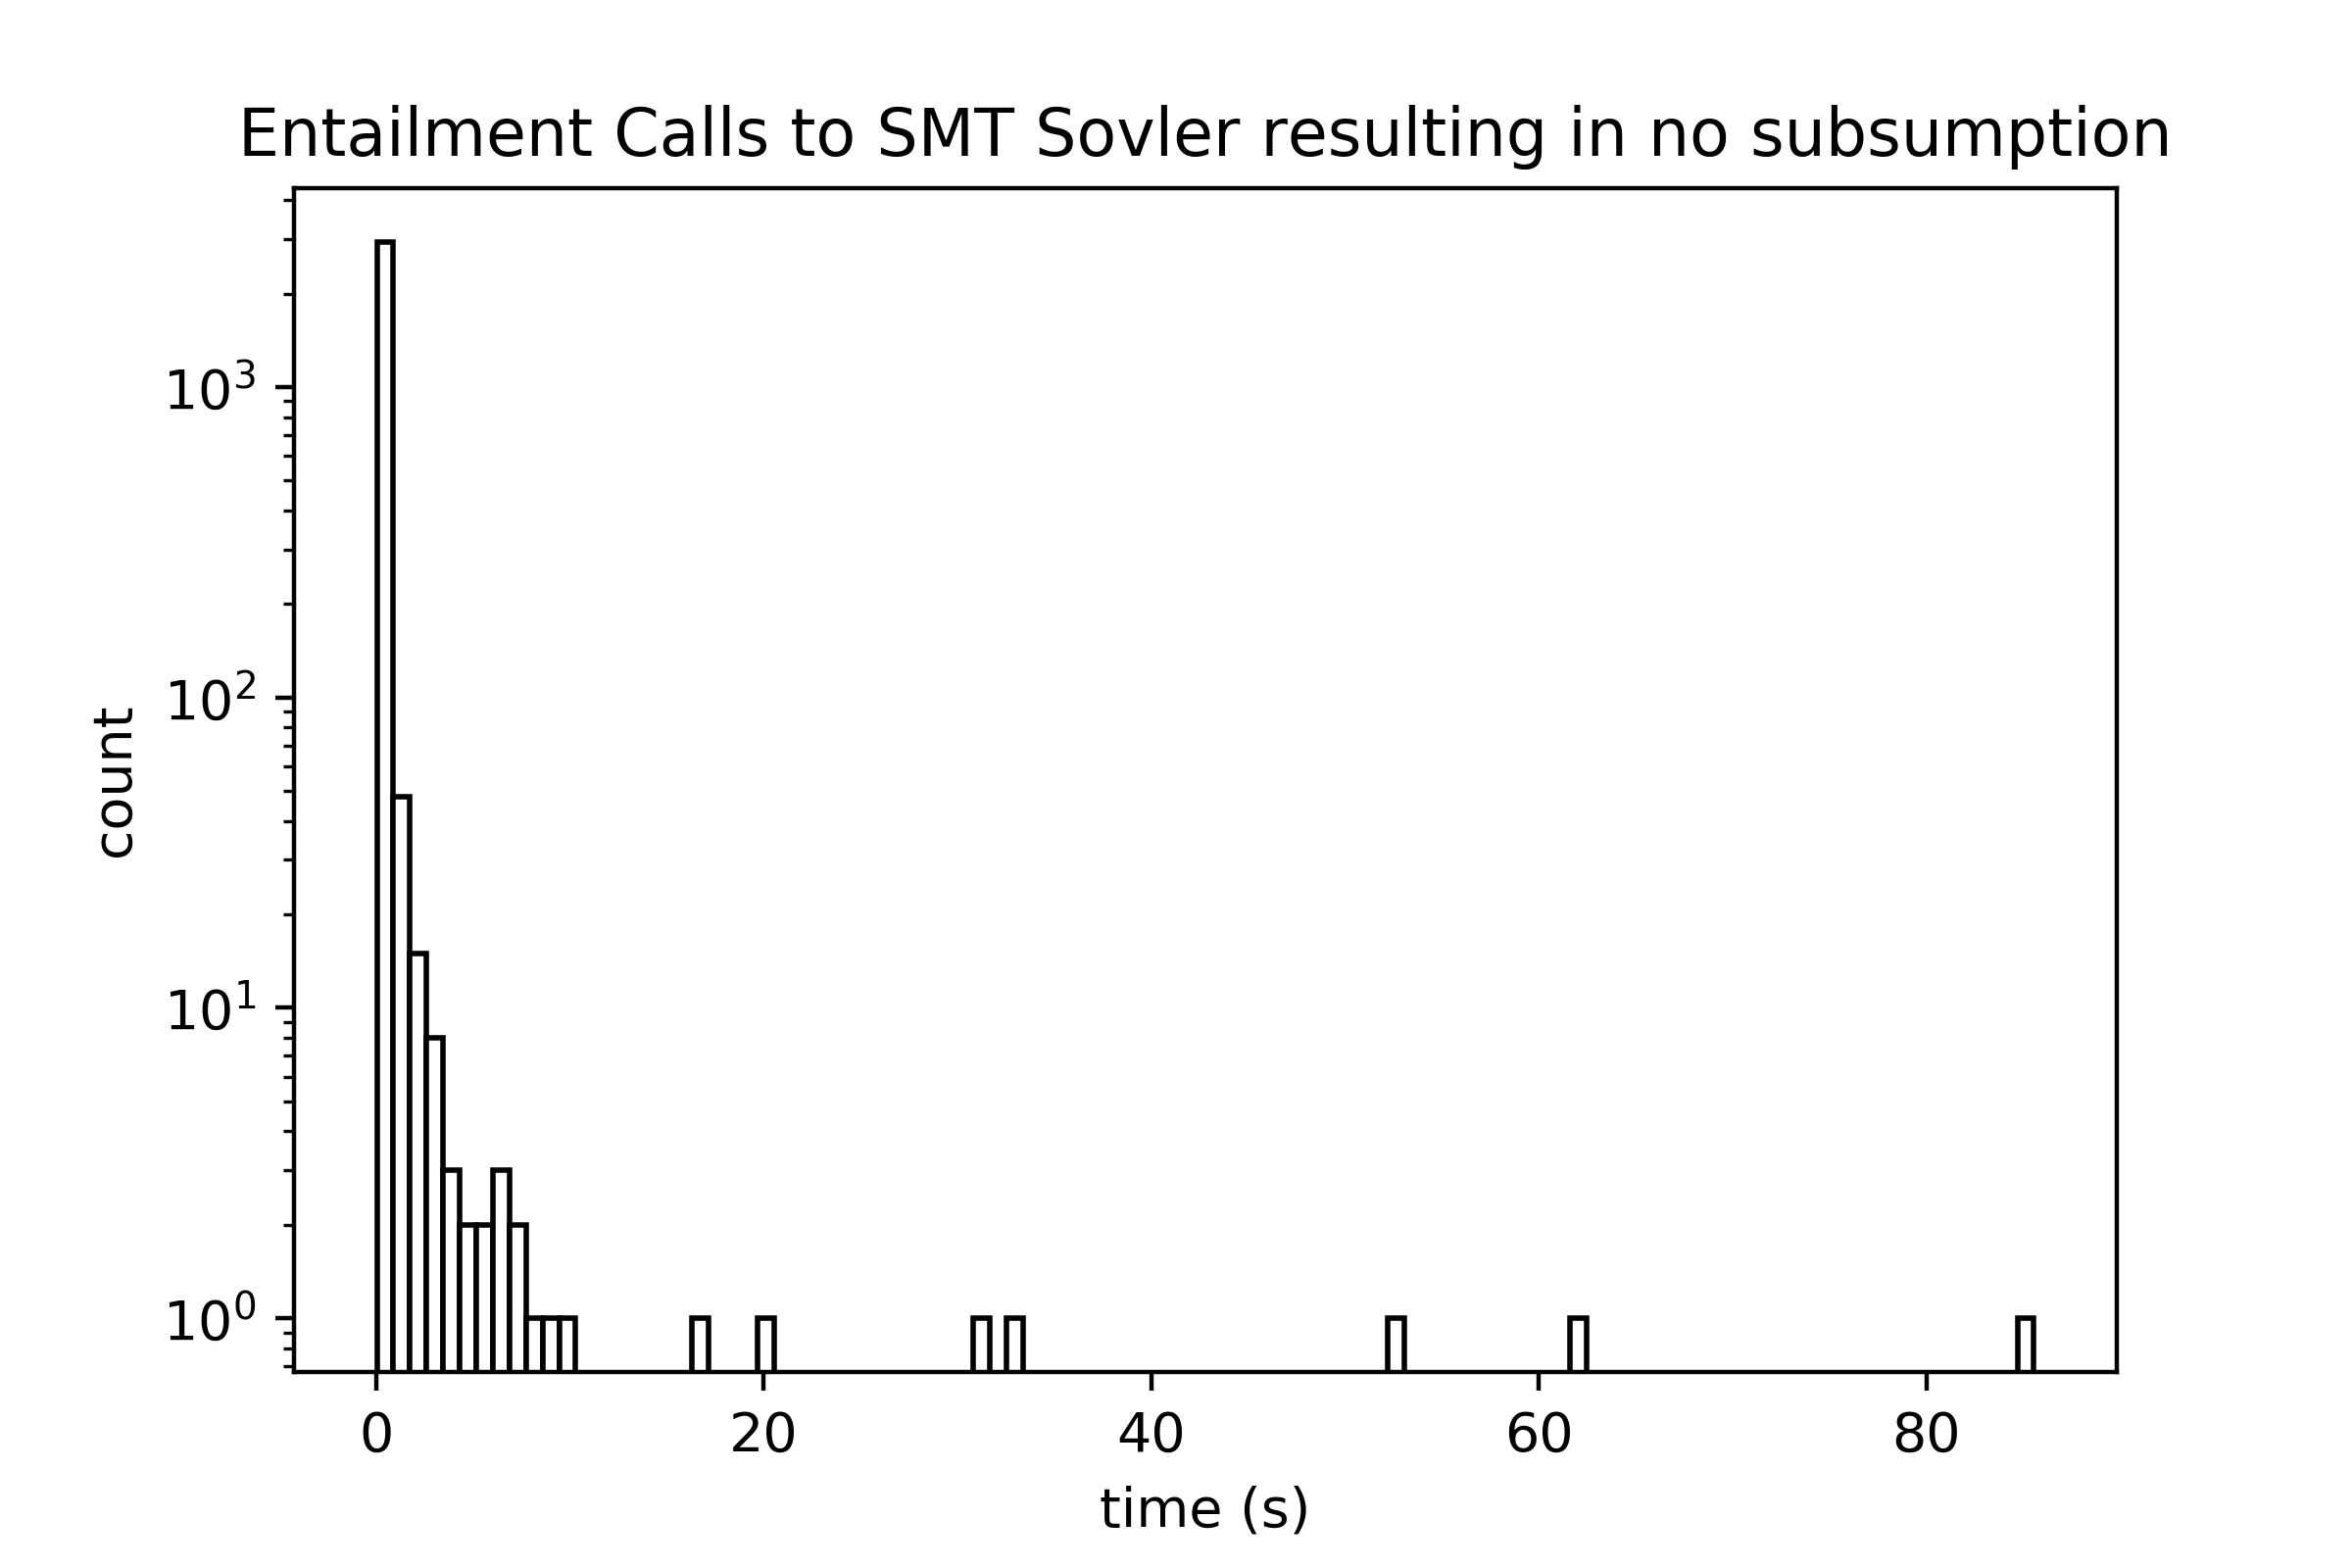}
\caption{Histograms of the time required for calls to the SMT solver for feasibility and entailment checks.}	
\end{figure}

\section{Weak points in the paper to improve}
Expressivity of cbcftl compared to other LTL
